# Supplementary material for: Follow-the-Perturbed-Leader for Adversarial Markov Decision Processes with Bandit Feedback
Source: arXiv:2205.13451 source file (2022-09-18)
Supplement: Supplementary file 1 [file appendix-geometric-resampling.tex]

%!TEX root=main.tex
